# Supplementary material for: Airflow recovery from thoracic and abdominal movements using Synchrosqueezing Transform and Locally Stationary Gaussian Process Regression
Source: arXiv:2008.04473 source file (2020-08-11)

Subject 1

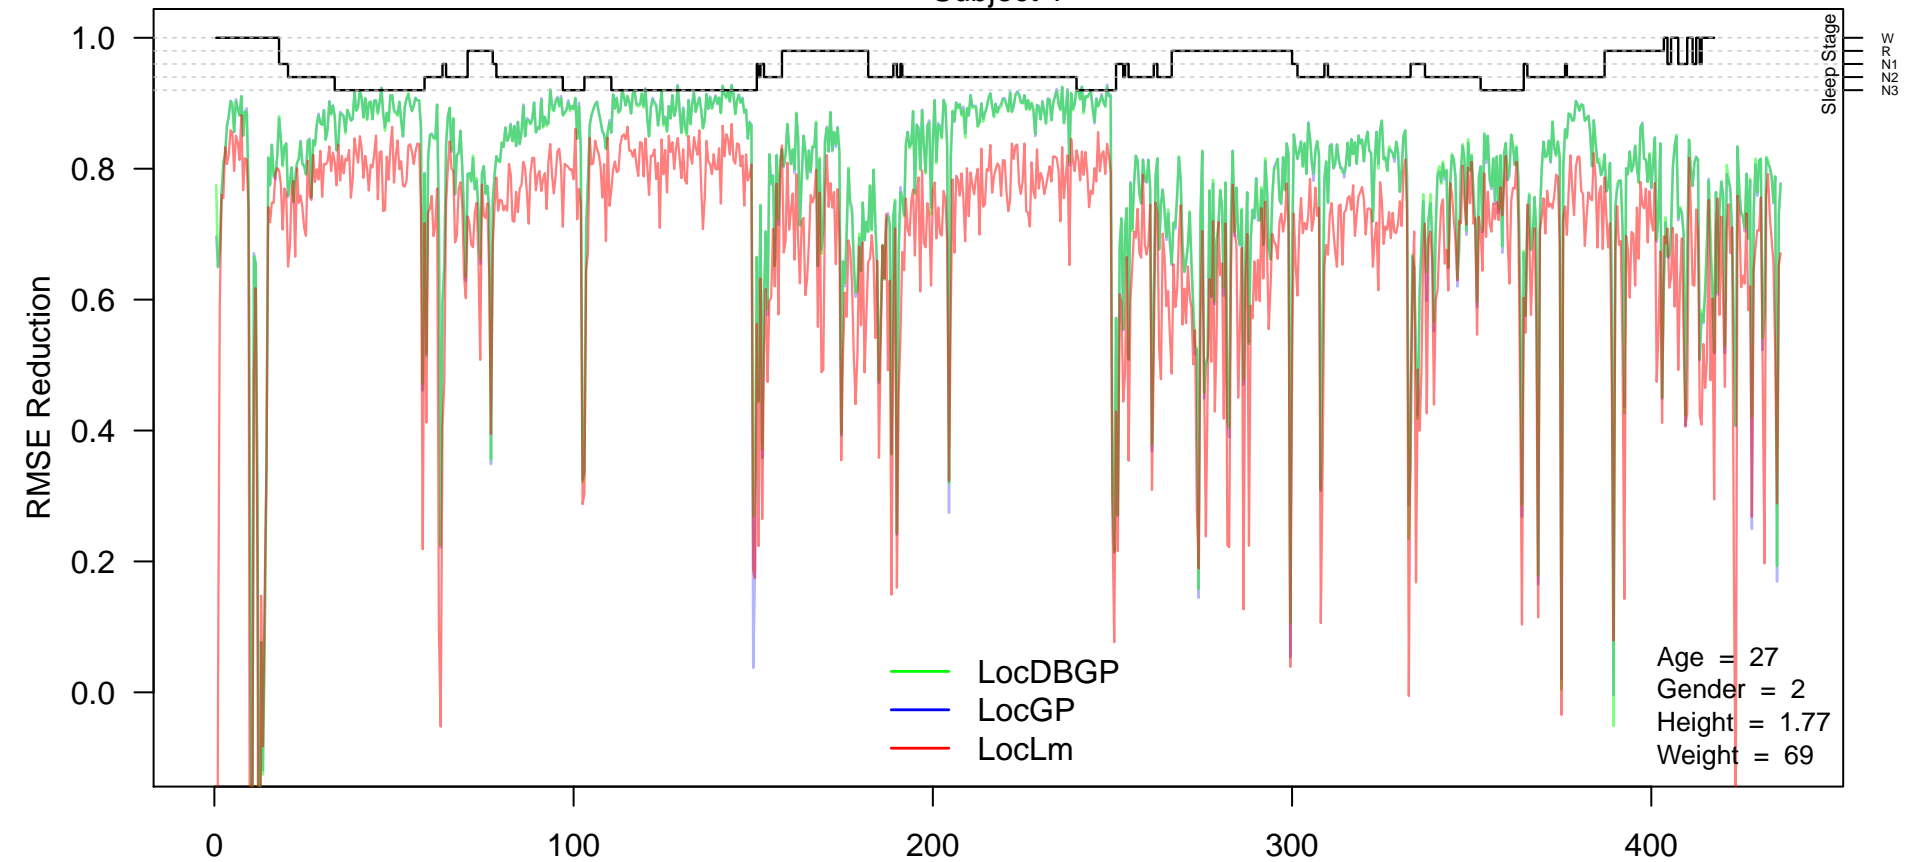

Subject 2

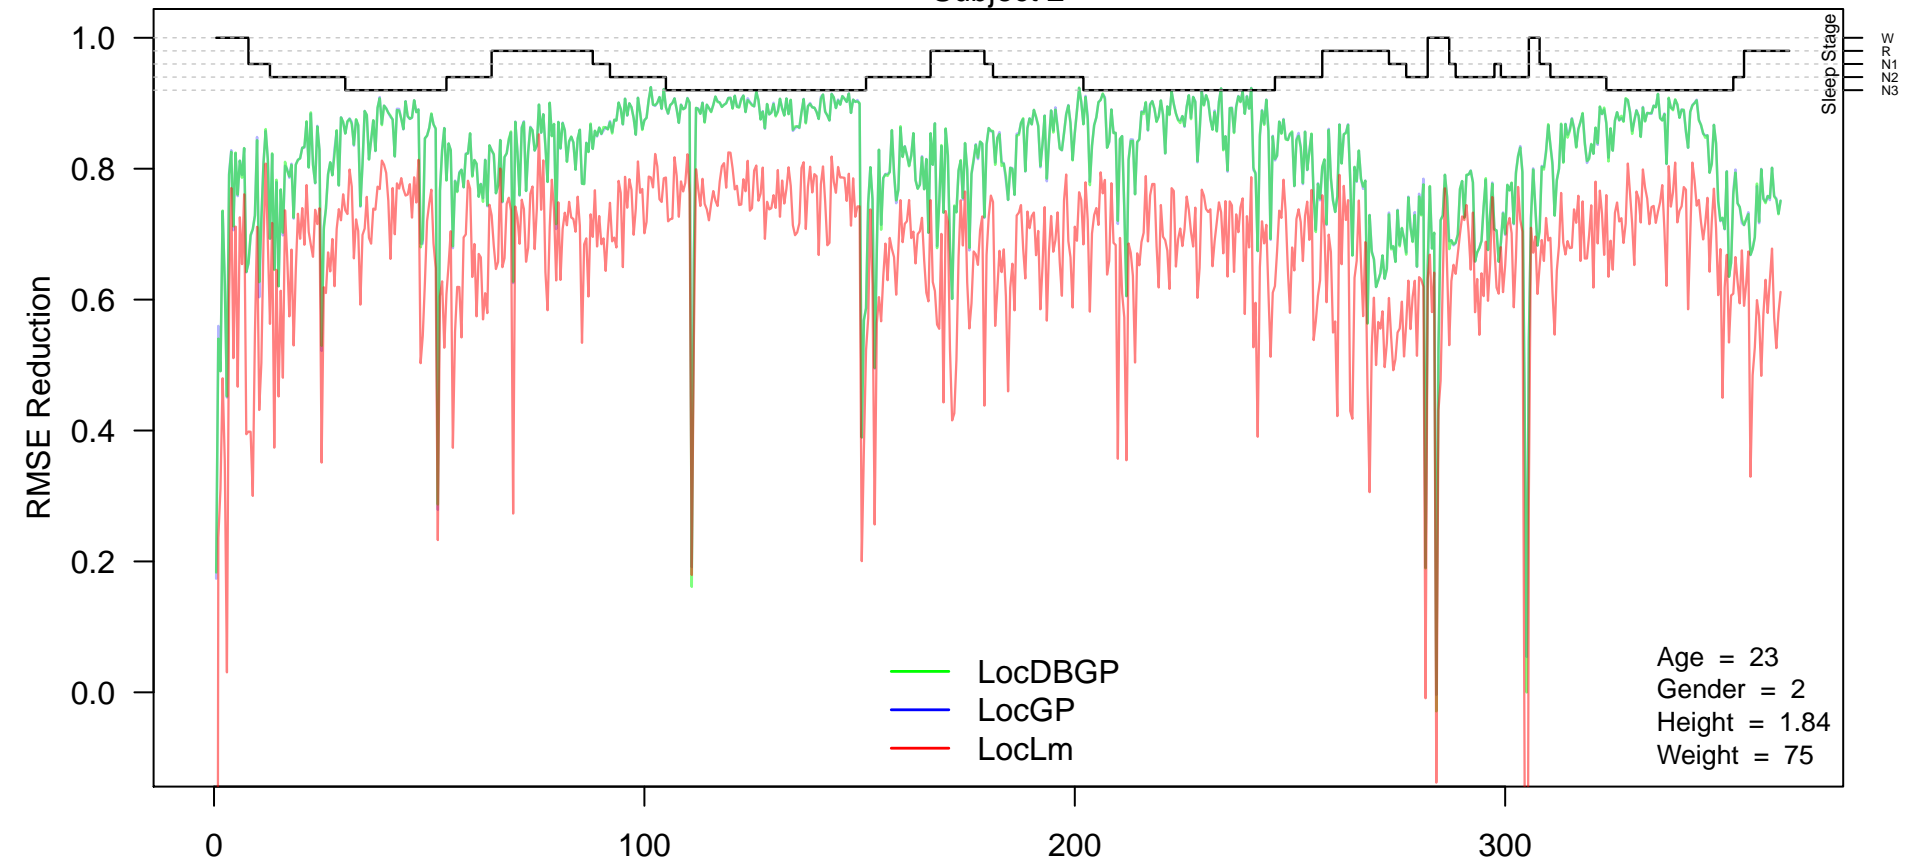

Subject 3

RMSE Reduction

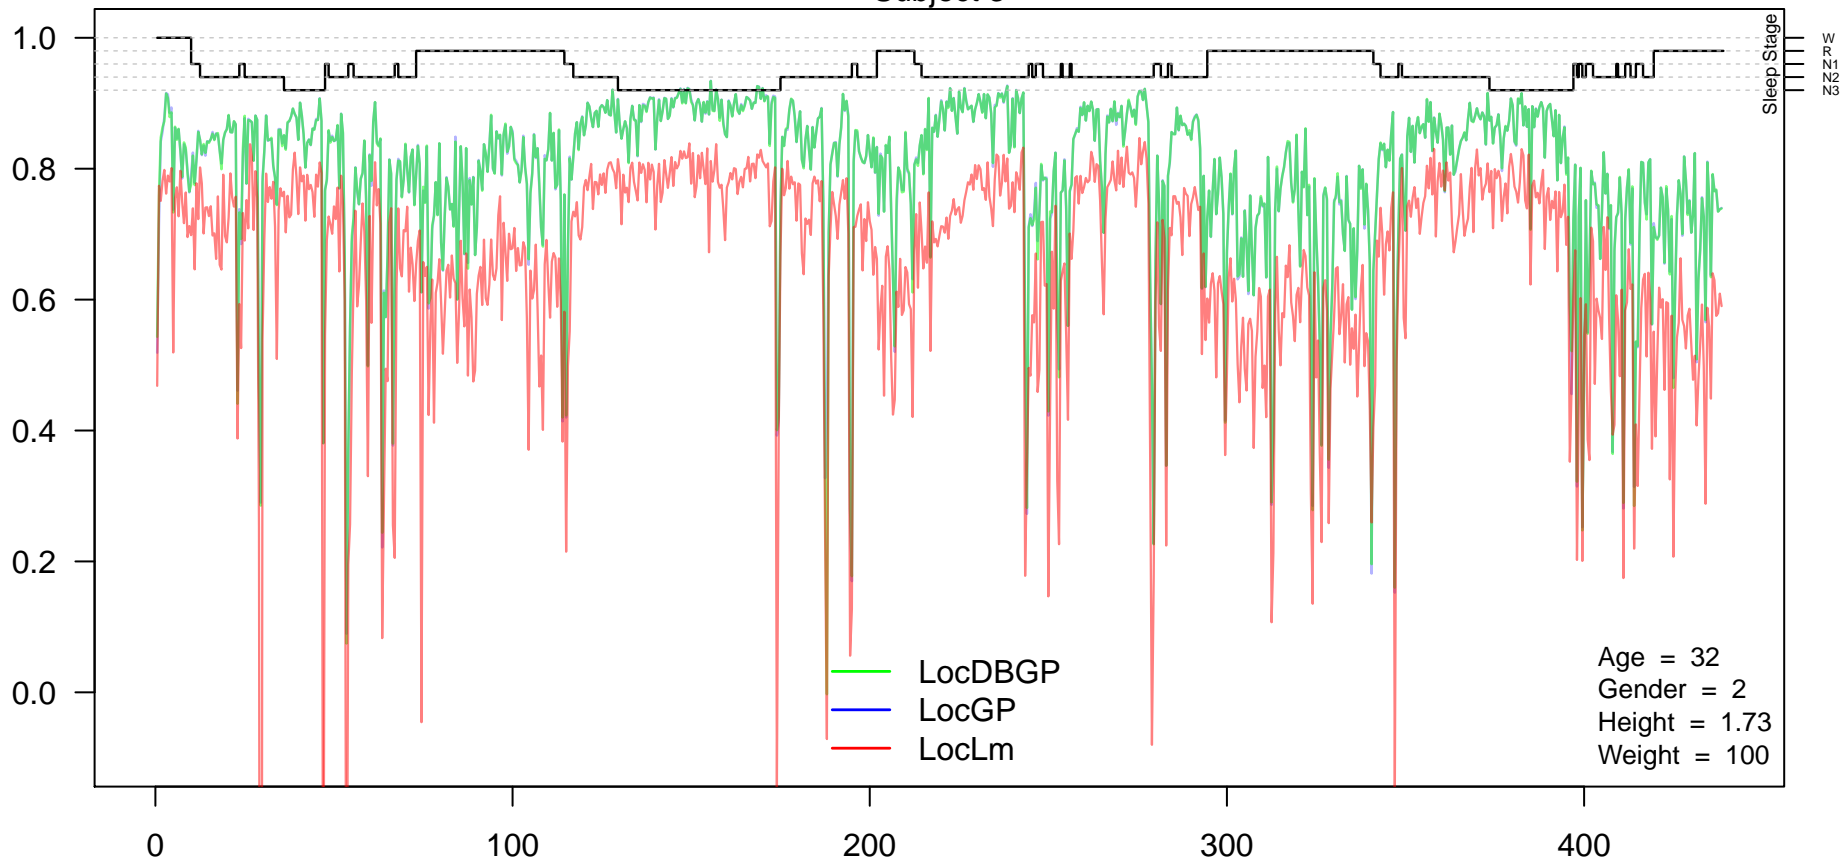

Subject 4

RMSE Reduction

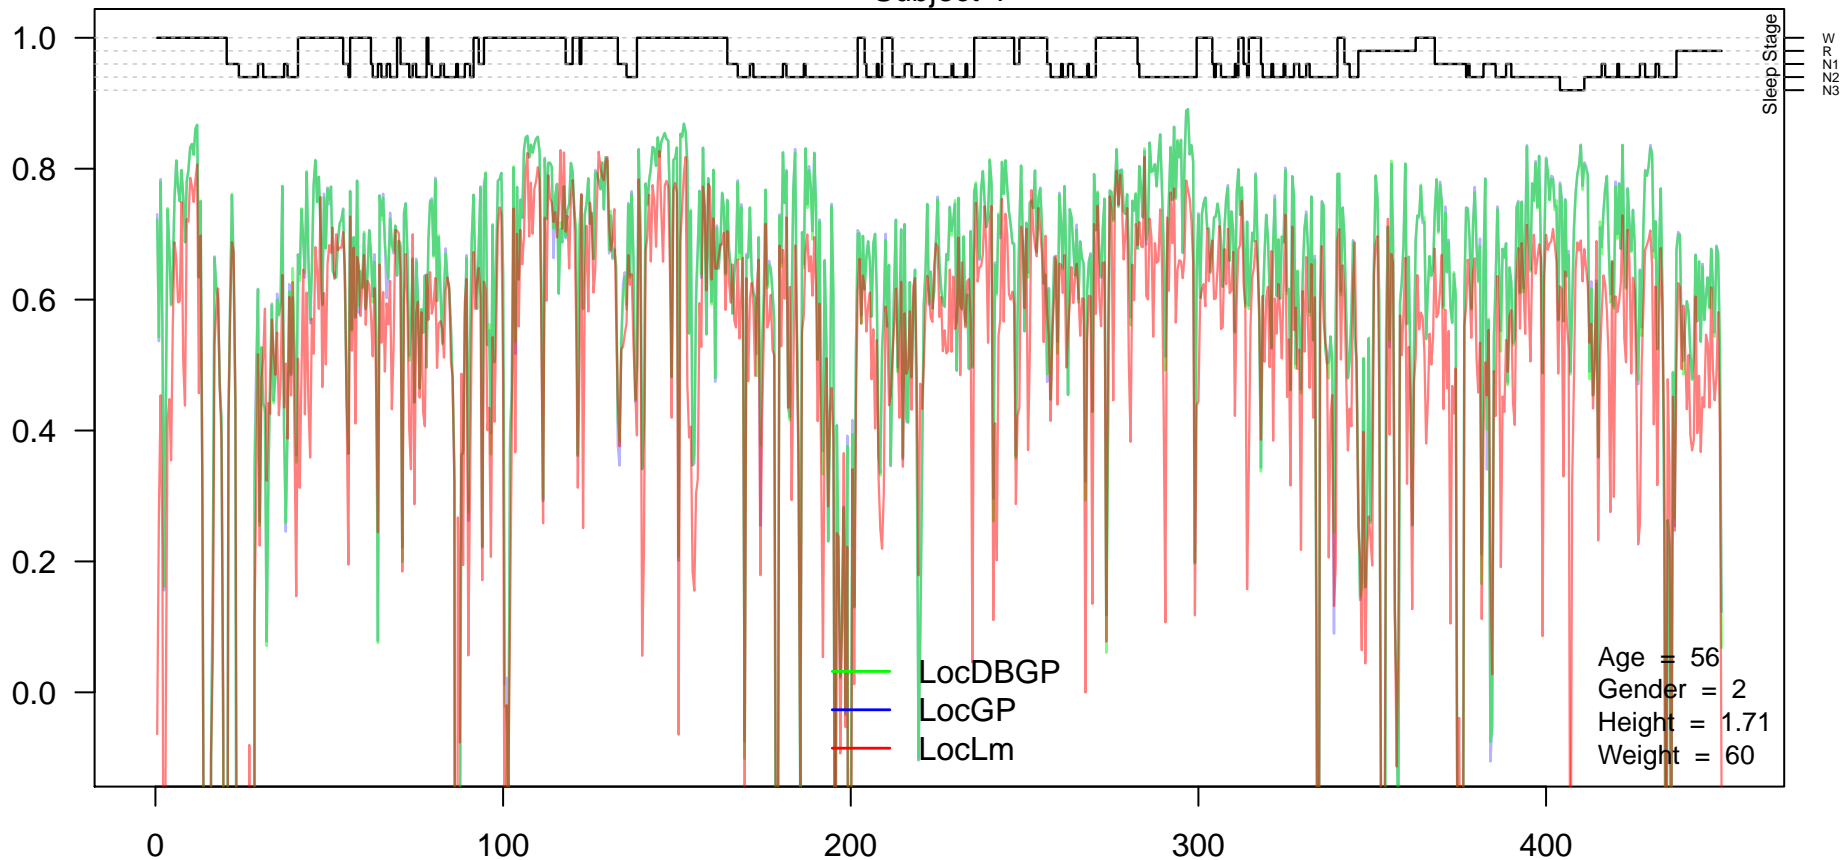

Subject 5

RMSE Reduction

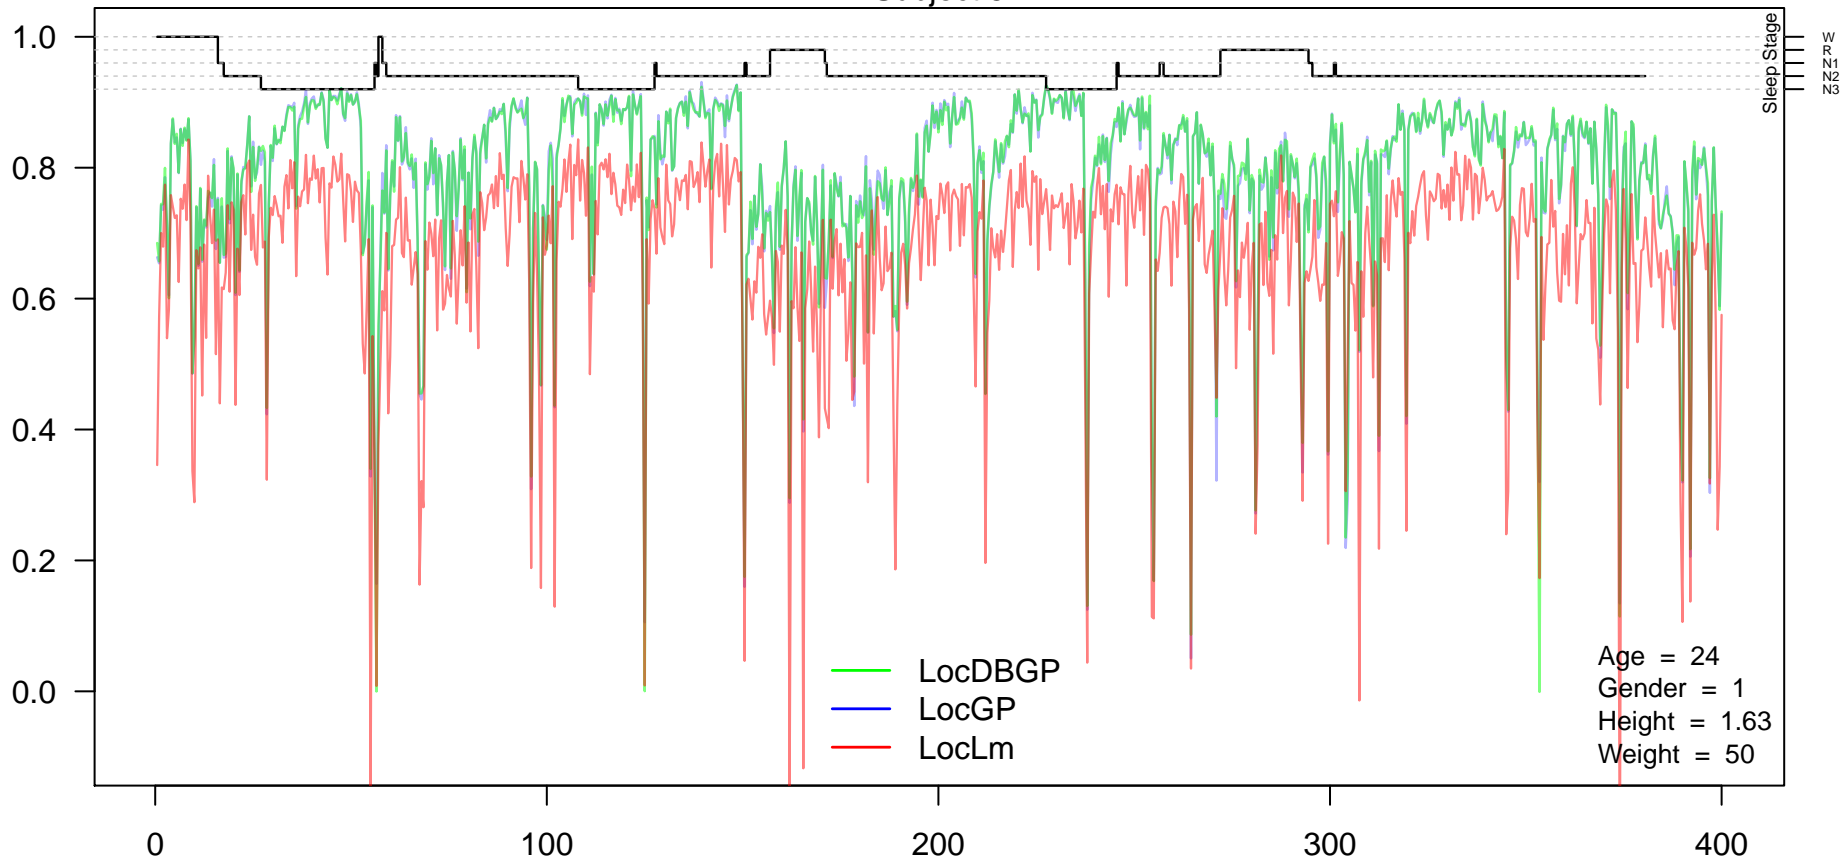

Supplement: Supplementary file 1 [file NNGPInRMSE_suppV2.pdf]
