# Supplementary material for: Airflow recovery from thoracic and abdominal movements using Synchrosqueezing Transform and Locally Stationary Gaussian Process Regression
Source: arXiv:2008.04473 source file (2020-08-11)

Subject 3

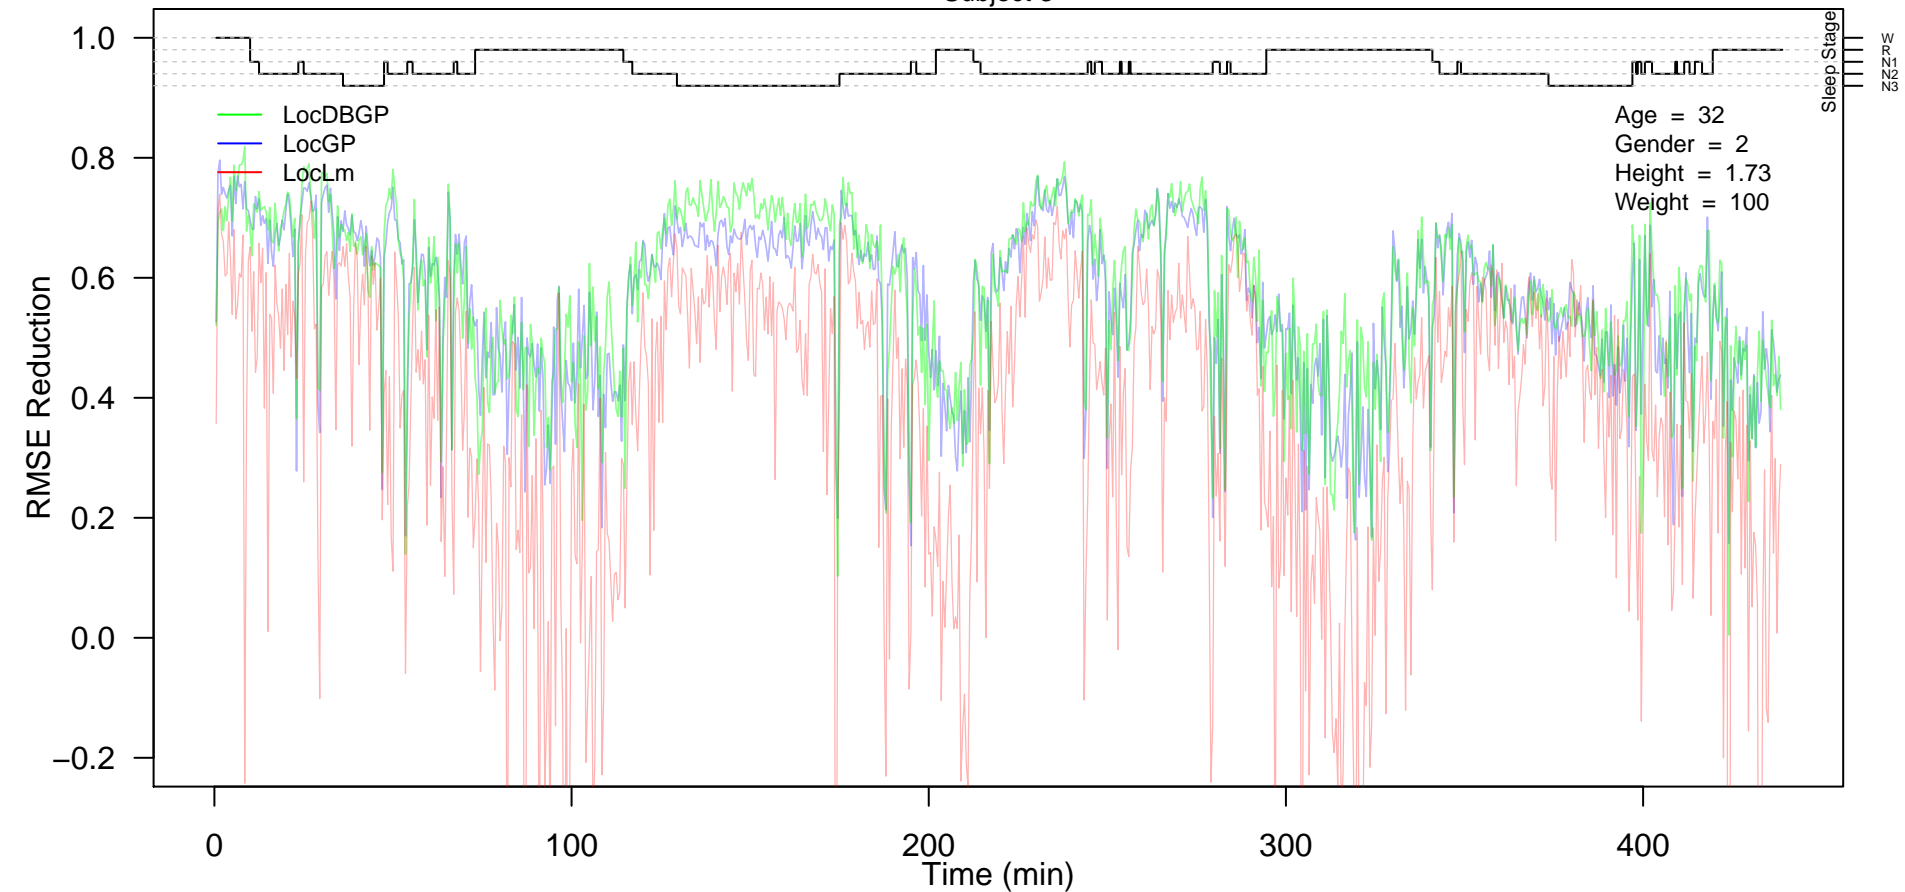

Subject 4

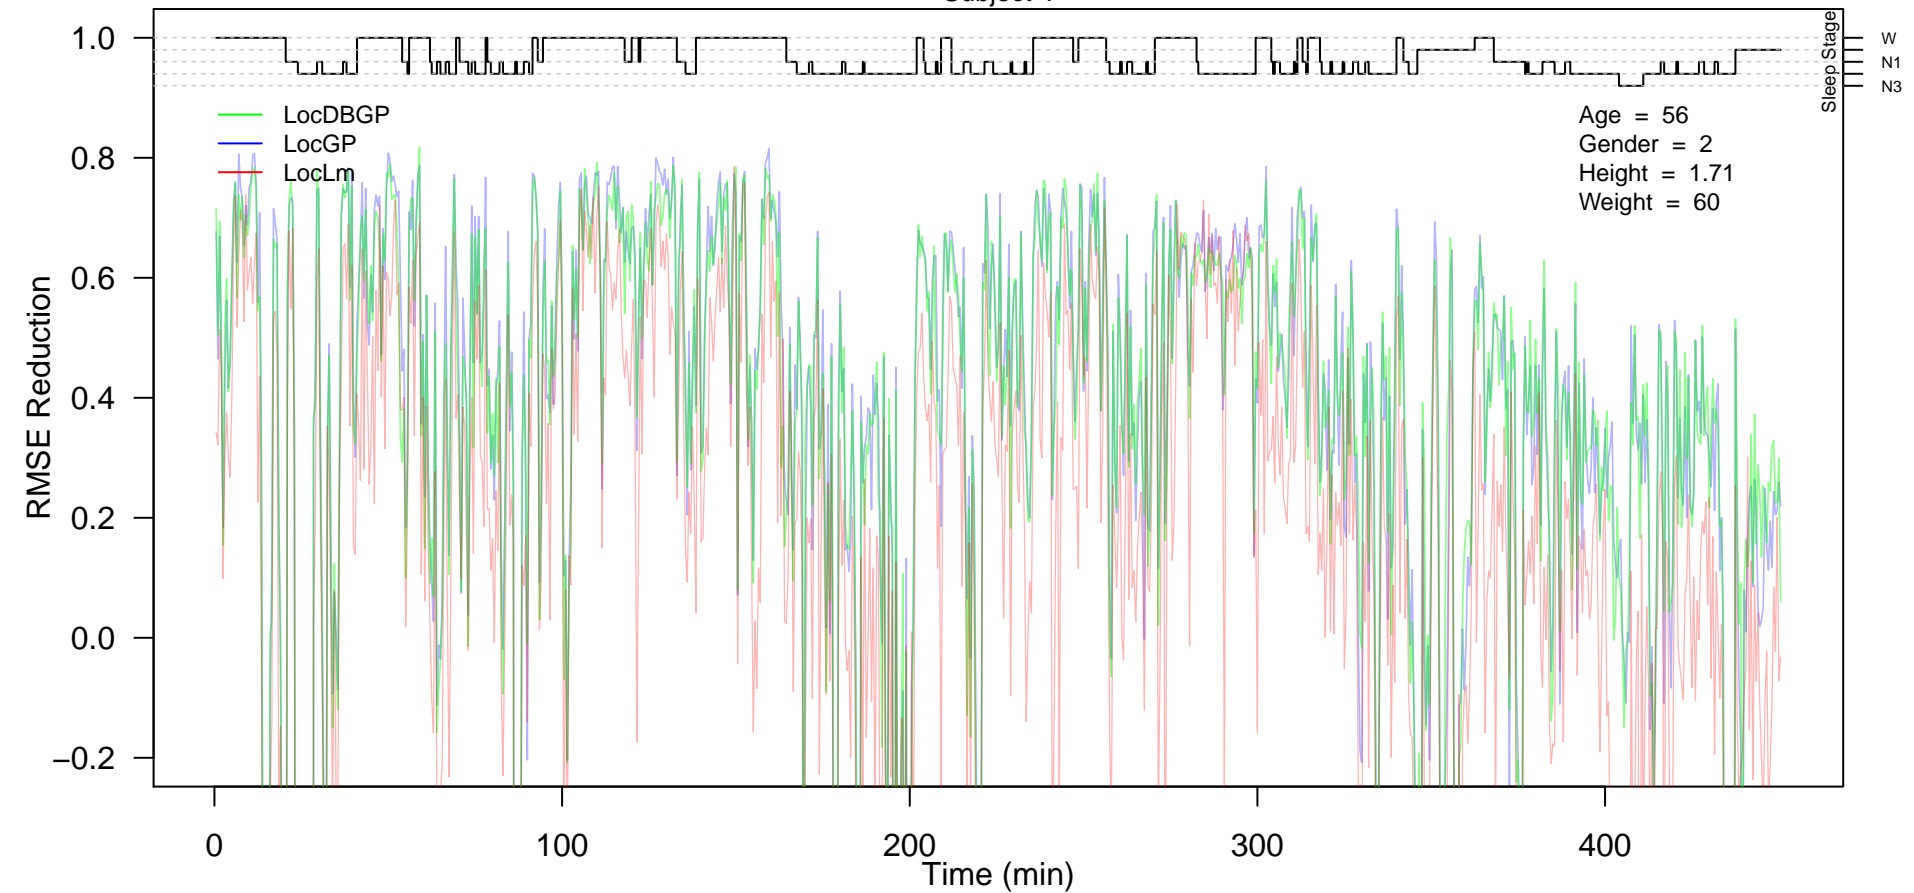

Subject 5

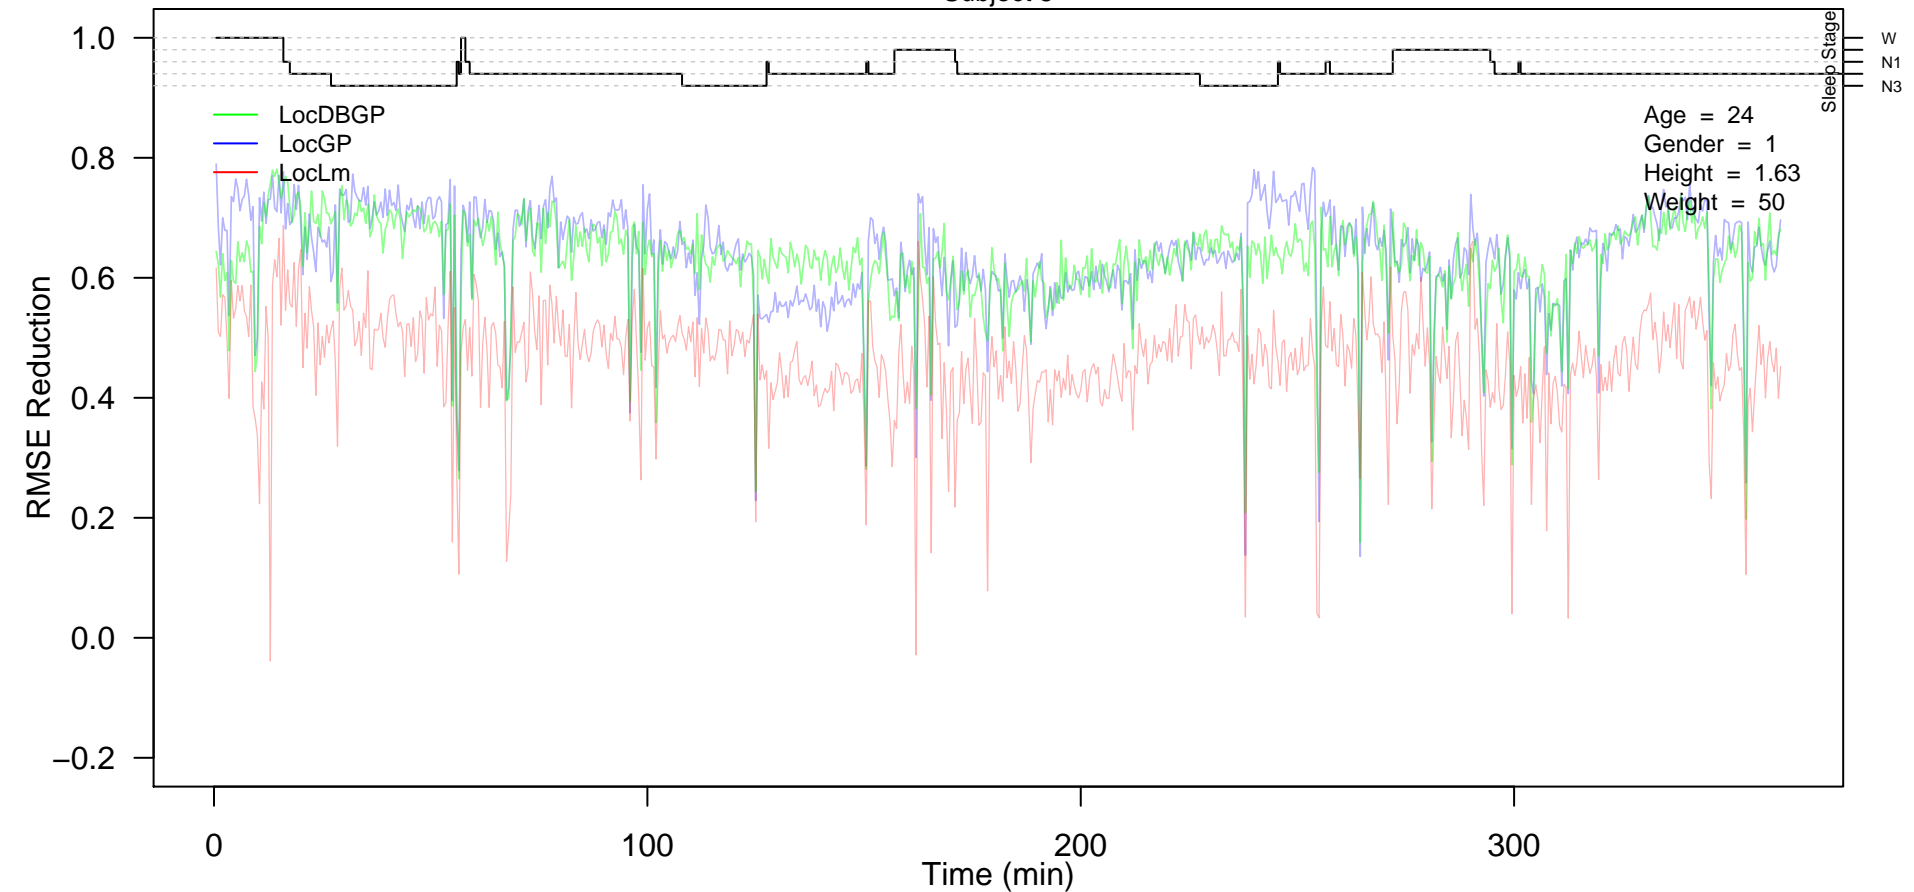

Supplement: Supplementary file 2 [file NNGPOutRMSE_suppV2.pdf]
